# Supplementary material for: Jump Restore Light Transport
Source: arXiv:2409.07148 source file (2025-10-10)
Supplement: Supplementary file 1 [file supplemental.tex]

\PassOptionsToPackage{hypertexnames = false}{hyperref}
\documentclass[acmtog]{acmart}

%% \BibTeX command to typeset BibTeX logo in the docs
\AtBeginDocument{%
  }

%% Rights management information.  This information is sent to you
%% when you complete the rights form.  These commands have SAMPLE
%% values in them; it is your responsibility as an author to replace
%% the commands and values with those provided to you when you
%% complete the rights form.
\setcopyright{rightsretained}
\acmJournal{TOG}
\acmYear{2025} \acmVolume{44} \acmNumber{6} \acmArticle{} \acmMonth{12} \acmPrice{}\acmDOI{10.1145/3763286}

%% Submission ID.
%% Use this when submitting an article to a sponsored event. You'll
%% receive a unique submission ID from the organizers
%% of the event, and this ID should be used as the parameter to this command.
\acmSubmissionID{1176}

\acmArticle{250}

% "too many math alphabets used in version normal":

\input{include}
\input{definition}

\begin{document}

\emergencystretch 3em

\title{Jump Restore Light Transport (Supplemental Material)}

%%
%% The "author" command and its associated commands are used to define
%% the authors and their affiliations.
%% Of note is the shared affiliation of the first two authors, and the
%% "authornote" and "authornotemark" commands
%% used to denote shared contribution to the research.
\author{Sascha Holl}
\authornote{Corresponding author.}
\email{sholl@mpi-inf.mpg.de}
\orcid{0009-0004-7245-7998}
\affiliation{%
  \institution{Max Planck Institute for Informatics}
  \city{Saarbrücken}
  \country{Germany}
}
\affiliation{%
  \institution{Saarland University}
  \city{Saarbrücken}
  \country{Germany}
}
% \homepage{https://people.mpi-inf.mpg.de/~sholl/}

\author{Gurprit Singh}
\email{gsingh@mpi-inf.mpg.de}
\orcid{0000-0003-0970-5835}
% \affiliation{%
%   \institution{Max Planck Institute for Informatics}
%   \city{Saarbrücken}
%   \country{Germany}
% }
\affiliation{%
  \institution{Advanced Micro Devices, Inc. (AMD)}
  \city{Saarbrücken}
  \country{Germany}
}
% \homepage{https://sampling.mpi-inf.mpg.de/}

\author{Hans-Peter Seidel}
\email{hpseidel@mpi-inf.mpg.de}
\orcid{0000-0002-1343-8613}
\affiliation{%
  \institution{Max Planck Institute for Informatics}
  \city{Saarbrücken}
  \country{Germany}
}
% \homepage{https://people.mpi-inf.mpg.de/~hpseidel/}
%%
%% By default, the full list of authors will be used in the page
%% headers. Often, this list is too long, and will overlap
%% other information printed in the page headers. This command allows
%% the author to define a more concise list
%% of authors' names for this purpose.
% \renewcommand{\shortauthors}{Trovato et al.}

%
% The code below should be generated by the tool at
% http://dl.acm.org/ccs.cfm
% Please copy and paste the code instead of the example below.
%
\begin{CCSXML}
<ccs2012>
   <concept>
       <concept_id>10002950.10003648</concept_id>
       <concept_desc>Mathematics of computing~Probability and statistics</concept_desc>
       <concept_significance>500</concept_significance>
       </concept>
   <concept>
       <concept_id>10002950.10003648.10003671</concept_id>
       <concept_desc>Mathematics of computing~Probabilistic algorithms</concept_desc>
       <concept_significance>500</concept_significance>
       </concept>
   <concept>
       <concept_id>10002950.10003648.10003700</concept_id>
       <concept_desc>Mathematics of computing~Stochastic processes</concept_desc>
       <concept_significance>500</concept_significance>
       </concept>
   <concept>
       <concept_id>10002950.10003648.10003700.10003701</concept_id>
       <concept_desc>Mathematics of computing~Markov processes</concept_desc>
       <concept_significance>500</concept_significance>
       </concept>
   <concept>
       <concept_id>10010147.10010371</concept_id>
       <concept_desc>Computing methodologies~Computer graphics</concept_desc>
       <concept_significance>500</concept_significance>
       </concept>
   <concept>
       <concept_id>10010147.10010371.10010372</concept_id>
       <concept_desc>Computing methodologies~Rendering</concept_desc>
       <concept_significance>500</concept_significance>
       </concept>
   <concept>
       <concept_id>10010147.10010371.10010372.10010374</concept_id>
       <concept_desc>Computing methodologies~Ray tracing</concept_desc>
       <concept_significance>500</concept_significance>
       </concept>
   <concept>
       <concept_id>10010147.10011777.10011778</concept_id>
       <concept_desc>Computing methodologies~Concurrent algorithms</concept_desc>
       <concept_significance>100</concept_significance>
       </concept>
 </ccs2012>
\end{CCSXML}

\ccsdesc[500]{Mathematics of computing~Probability and statistics}
\ccsdesc[500]{Mathematics of computing~Probabilistic algorithms}
\ccsdesc[500]{Mathematics of computing~Stochastic processes}
\ccsdesc[500]{Mathematics of computing~Markov processes}
\ccsdesc[500]{Computing methodologies~Computer graphics}
\ccsdesc[500]{Computing methodologies~Rendering}
\ccsdesc[500]{Computing methodologies~Ray tracing}
\ccsdesc[100]{Computing methodologies~Concurrent algorithms}

%
% End generated code
%

\keywords{diffusion processes, jump-type Markov processes, light transport simulation}

\maketitle

\appendix

\section{Invariance of the Restore process}\label{sec:invariance-proof}

The process $\concatenatedprocess$ constructed in Section 6 of the main paper is \emph{locally} (during a single tour) a \emph{jump-type Markov process}. In general, such a process is a Markov process $(\concatenatedprocess_\timepoint)_{\timepoint\ge0}$ with values in a measurable space $(\measurablespace,\measurablesystem)$ and a generator (see Section 3.2.3 of the main paper) of the form \begin{equation}
    \concatenatedgenerator\integrand:=\localgenerator\integrand+\killingrate\globalgenerator\integrand\;\;\;\text{for }\integrand\in\mathcal D(\localgenerator).
\end{equation} where $\localgenerator$ is the generator of a Markov semigroup $(\localsemigroup_\timepoint)_{\timepoint\ge0}$ on $(\measurablespace,\measurablesystem)$, $\killingrate:\measurablespace\to[0,\infty)$ is $\measurablesystem$-measurable and $\regenerationdistribution$ is a Markov kernel on $(\measurablespace,\measurablesystem)$. $\killingrate$, $\regenerationdistribution$ and \begin{equation}
    \ratekernel(\point,\measurableset):=\killingrate(\point)\regenerationdistribution(\point,\measurableset)\;\;\;\text{for }(\point,\measurableset)\in\measurablespace\times\measurablesystem
\end{equation} are called \emph{rate function}, \emph{jump transition kernel} and \emph{rate kernel} of $(\concatenatedprocess_\timepoint)_{\timepoint\ge0}$, respectively.
The terminology is intuitive: A transition according to $\ratekernel$ is happening with rate $\killingrate$ and is performed by following $\regenerationdistribution$. For a general discussion on such processes, we refer to \citet[Chapter~13]{kallenberg2021probability}.

Given a probability measure $\targetdistribution$ on $(\measurablespace,\measurablesystem)$, our goal in this section is to derive a choice for the rate function $\killingrate$ for which the process $(\concatenatedprocess_\timepoint)_{\timepoint\ge0}$ is $\targetdistribution$-invariant. The result obtained this way will immediately give the right choice of killing rates for the Restore process defined in Equation 20 of the main paper.

The following assumption can be relaxed, but it simplifies the analysis and is already in place in our setting in Section 6 of the main paper. We assume, for the remainder of this section, that both, the regeneration kernel $\regenerationdistribution$ and the target distribution $\targetdistribution$, have a density with respect to a common $\sigma$-finite reference measure $\referencemeasure$ on $(\measurablespace,\measurablesystem)$. To be precise, we assume that there is a $\measurablesystem$-measurable $\targetdensity:\measurablespace\to(0,\infty)$ with \begin{equation}
    \targetdensity_\referencemeasure:=\referencemeasure\targetdensity\in(0,\infty)
\end{equation} and \begin{equation}
    \targetdistribution=\frac\targetdensity{\targetdensity_\referencemeasure}\referencemeasure.
\end{equation} Analogously, we assume that there is an $\measurablesystem^{\otimes2}$-measurable $\regenerationdensity:\measurablespace^2\to[0,\infty)$ with \begin{equation}
    \regenerationdensity_\referencemeasure(\point):=\referencemeasure\regenerationdensity(\point,\;\cdot\;)\in(0,\infty)
\end{equation} and \begin{equation}
    \regenerationdistribution(\point,\;\cdot\;)=\frac{\regenerationdensity(\point,\;\cdot\;)}{\regenerationdensity_\referencemeasure(\point)}\referencemeasure.
\end{equation} for all $\point\in\measurablespace$.
If $\genericoperator$ is an operator on $\measurablesystem_b$, we denote the $\referencemeasure$-adjoint of $\genericoperator$, defined in Section 3.2.4 of the main paper, by $\genericoperator^\ast$. We are now able to state and proof the main theorem of this section:

\begin{theorem}\label{thm:restore-process-invariance}
    \normalfont If $\targetdensity\in\mathcal D(\localgenerator^\ast)$ with \begin{equation}\label{eq:restore-process-invariance-eq1}
        \referencemeasure\left(\regenerationdistribution^\ast\localgenerator^\ast\targetdensity\right)=0
    \end{equation} and \begin{equation}\label{eq:restore-process-invariance-eq2}
        \killingrate=\frac{\left(\expectedlifetime_1\regenerationdistribution^\ast+\localgenerator^\ast\right)\targetdensity}\targetdensity
    \end{equation}
    % \begin{alignat}{2}\label{eq:restore-process-invariance-eq2}
    %     \killingrate&=\frac{\left(\expectedlifetime_1\regenerationdistribution^\ast+\localgenerator^\ast\right)\targetdensity}\targetdensity&\;\;\;\text{on }\{\;\targetdensity>0\;\}\\
    %     \killingrate&=\infty&\;\;\;\text{on }\{\;\targetdensity=0\;\}
    % \end{alignat}
    for some $\expectedlifetime_1\ge0$, then \begin{equation}
        \targetdistribution\concatenatedgenerator\integrand=0\;\;\;\text{for all }\integrand\in\mathcal D(\concatenatedgenerator).
    \end{equation}
    \begin{proof}[Proof\textup:\nopunct]
        Let $\integrand\in\mathcal D(\localgenerator)$. By \eqref{eq:restore-process-invariance-eq1}, \begin{equation}
            \begin{split}
                \left|\left\langle\regenerationdistribution\integrand,\localgenerator^\ast\targetdensity\right\rangle_\referencemeasure\right|&=\left|\left\langle\integrand,\regenerationdistribution^\ast\localgenerator^\ast\targetdensity\right\rangle_\referencemeasure\right|\\&\le\left\|\integrand\right\|_\infty\underbrace{\referencemeasure\left(\regenerationdistribution^\ast\localgenerator^\ast\targetdensity\right)}_{=\:0}=0
            \end{split}
        \end{equation} and hence \begin{equation}
            \referencemeasure\left(\targetdensity\ratekernel\integrand\right)=\underbrace{\left\langle\regenerationdistribution\integrand,\localgenerator^\ast\targetdensity\right\rangle_\referencemeasure}_{=\:0}+\:\expectedlifetime_1\left\langle\regenerationdistribution\integrand,\regenerationdistribution^\ast\targetdensity\right\rangle_\referencemeasure
        \end{equation} by \eqref{eq:restore-process-invariance-eq2}. Again by \eqref{eq:restore-process-invariance-eq2}, we obtain \begin{equation}
            \begin{split}
                \referencemeasure\left(\targetdensity\killingrate\integrand\right)&=\left\langle\integrand,\left(\localgenerator^\ast+\expectedlifetime_1\regenerationdistribution^\ast\right)\targetdensity\right\rangle_\referencemeasure\\&=\left\langle\left(\localgenerator+\expectedlifetime_1\regenerationdistribution\right)\integrand,\targetdensity\right\rangle_\referencemeasure
            \end{split}
        \end{equation} and hence \begin{equation}
            \begin{split}
                \targetdensity_\referencemeasure\targetdistribution\localgenerator\integrand&=\referencemeasure\left(\targetdensity\localgenerator\integrand\right)-\referencemeasure\left(\targetdensity\killingrate\integrand\right)+\referencemeasure\left(\targetdensity\ratekernel\integrand\right)\\&=\expectedlifetime_1\left\langle\regenerationdistribution\integrand,\tilde\localgenerator^\ast\targetdensity\right\rangle_\referencemeasure=0.
            \end{split}
        \end{equation} For the last equation, note that $\globalgenerator^\ast=\regenerationdistribution^\ast-\operatorname{id}_{\measurablesystem_b}$ and $\globalgenerator1=0$.
        % \begin{equation}
        %     \globalgenerator^\ast=\regenerationdistribution^\ast-\operatorname{id}_{\measurablesystem_b}
        % \end{equation} and \begin{equation}
        %     \globalgenerator1=0.
        % \end{equation}
    \end{proof}
\end{theorem}

A crucial condition, which is implicit in \eqref{eq:restore-process-invariance-eq2}, is that $\expectedlifetime_1$ must be large enough to ensure $\killingrate\ge0$. If $(\localsemigroup_\timepoint)_{\timepoint\ge0}$ is already $\targetdistribution$-invariant, then $\localgenerator^\ast\targetdensity=0$ (see Section 3.2.4 of the main paper) and hence condition \eqref{eq:restore-process-invariance-eq2} is reduced to \begin{equation}
    \killingrate=\expectedlifetime_1\frac{\regenerationdistribution^\ast\targetdensity}\targetdensity
\end{equation} In that case, $\expectedlifetime_1$ can be arbitrary. If $\targetdistribution$ is state-independent (i.e. does not depend on the first argument and hence is simply a measure), then the adjoint of $\targetdistribution$ is given by \begin{equation}
    \regenerationdistribution^\ast\secondintegrand=\frac{\referencemeasure\secondintegrand}{\regenerationdensity_\referencemeasure}\regenerationdensity\eqforall\secondintegrand\in\mathcal L^1(\referencemeasure)
\end{equation} and hence condition \eqref{eq:restore-process-invariance-eq2} actually is \begin{equation}
    \killingrate=\frac{\displaystyle\expectedlifetime_1\frac{\targetdensity_\referencemeasure}{\regenerationdensity_\referencemeasure}\regenerationdensity+\localgenerator^\ast\targetdensity}\targetdensity.
\end{equation}

\section{Theoretical convergence investigation}\label{sec:convergence-analysis}

Our goal in this section is to compare the quality of an estimation based on \begin{enumerate}
    \item the \gls{mh} chain $\markovchain^\largestepprobability$ with proposal kernel $\proposalkernel_\largestepprobability$ and target distribution $\targetdistribution$; and
    \item the process $\concatenatedprocess$ formed by the jump Restore algorithm with local dynamics $\markovchain^0$ and regeneration distribution $\regenerationdistribution$.
\end{enumerate} The generators $\localgenerator_\largestepprobability$ and $\concatenatedgenerator$ of $\markovchain^\largestepprobability$ and $\concatenatedprocess$ will play an important role in the theoretical investigation of this comparison.

% The $L^2$\emph{-relaxation time} \citep[eq.~15]{eberle2024relaxation} of a time-homogeneous Markov process $(\concatenatedprocess_\timepoint)_{\timepoint\ge0}$ with invariant measure $\targetdistribution$ is governed by the \emph{spectral gap} \begin{equation}
%     \operatorname{gap}(\genericgenerator):=\inf\left\{\frac{\dirichletform(\integrand)}{\left\|\integrand\right\|_{L^2(\targetdistribution}^2}:\integrand\in\mathcal D(\genericgenerator)\setminus\{0\}\text{ with }\targetdistribution\integrand=0\right\}.
% \end{equation} of its $L^2(\targetdistribution)$-generator $\genericgenerator$. Here, \begin{equation}
%     \dirichletform(\integrand,\secondintegrand):=-\langle\genericgenerator\integrand,\secondintegrand\rangle_{L^2(\targetdistribution)}\;\;\;\text{for }\integrand\in\mathcal D(\genericgenerator)\text{ and }\secondintegrand\in L^2(\targetdistribution)
% \end{equation} is the \emph{Dirichlet form} associated with $\genericgenerator$ and $\dirichletform(\integrand):=\dirichletform(\integrand,\integrand)$ for $\integrand\in\mathcal D(\genericgenerator)$.

Our measure of quality will be based on the \emph{asymptotic variance}. If $\integrand\in L^2(\targetdistribution)$, we can define the asymptotic variance \begin{equation}
    \sigma^2_\concatenatedgenerator(\integrand):=\lim_{\timepoint\to\infty}\operatorname{Var}_\targetdistribution\left[\frac1{\sqrt\timepoint}\int_0^\timepoint\integrand(\concatenatedprocess_\timepoint)\dif\timepoint\right]
\end{equation} of the ergodic average estimation of $\targetdistribution\integrand$ based on $\concatenatedprocess$, whenever the limit exists. In that case, the ergodic average (defined in Equation 2 of the main paper) is asymptotically behaving as $\sigma^2_\genericgenerator(\integrand)/\timepoint$. Here, the variance is taken with respect to the probability measure with respect to which the initial distribution of $\concatenatedprocess$ is already $\targetdistribution$. That is, the assumption in this consideration is that the process is started in stationarity.

In the $L^2(\targetdistribution)$-reversible case, the $L^2$\emph{-relaxation time} \citep[Section~3]{eberle2024relaxation} of a time-homogeneous Markov process $\concatenatedprocess$ with invariant measure $\targetdistribution$ is governed by the \emph{spectral gap} \begin{equation}
    \operatorname{gap}(\genericgenerator):=\inf\left\{\frac{\dirichletform(\integrand)}{\left\|\integrand\right\|_{L^2(\targetdistribution)}^2}:\integrand\in\mathcal D(\genericgenerator)\setminus\{0\}\text{ with }\targetdistribution\integrand=0\right\}.
\end{equation} of its $L^2(\targetdistribution)$-generator $\genericgenerator$. Here, \begin{equation}
    \dirichletform(\integrand,\secondintegrand):=-\langle\genericgenerator\integrand,\secondintegrand\rangle_{L^2(\targetdistribution)}\;\;\;\text{for }\integrand\in\mathcal D(\genericgenerator)\text{ and }\secondintegrand\in L^2(\targetdistribution)
\end{equation} is the \emph{Dirichlet form} associated with $\genericgenerator$ and \begin{equation}
    \dirichletform(\integrand):=\dirichletform(\integrand,\integrand)\eqfor\integrand\in\mathcal D(\genericgenerator).
\end{equation} In the general, non-$L^2(\targetdistribution)$-reversible, case, the $L^2$-relaxation time is at least still lower bounded by $\operatorname{gap}(\genericgenerator)$.

However, similar to the celebrated \emph{Peskun-Tierney ordering}, we can show \citep{andrieu2019ordering} that an ordering \begin{equation}\label{eq:dirichlet-form-ordering}
    \dirichletform_\largestepprobability(\integrand)\le\dirichletform(\integrand)\eqforall\integrand\in\measurablesystem_b
\end{equation} on the Dirichlet forms $\dirichletform_\largestepprobability$ and $\dirichletform$ of $\concatenatedprocess$ and $\markovchain^\largestepprobability$, respectively, directly corresponds to an ordering \begin{equation}
    \sigma^2_{\localgenerator_\largestepprobability}(\integrand)\ge\sigma^2_\concatenatedgenerator(\integrand)
\end{equation} of the asymptotic variances of the corresponding ergodic averages.

We still can compare the performance of different processes by considering the asymptotic variances of their ergodic averages. Similar to the celebrated \emph{Peskun-Tierney ordering} \citep{tierney1998note}, an ordering among asymptotic variances is directly related to an ordering of the corresponding \emph{Dirichlet forms} \citep{andrieu2019ordering}. 

That is, we can compare the asymptotic variances of $\markovchain^\largestepprobability$ and $\concatenatedprocess$ by proving that their corresponding Dirichlet forms $\dirichletform_\largestepprobability$ and $\dirichletform$ are ordered. We are actually able to do so:

\begin{theorem}
    \normalfont If \begin{equation}
        \expectedlifetime_1\ge\frac\largestepprobability{2\targetdensity_\referencemeasure},
    \end{equation} then \eqref{eq:dirichlet-form-ordering} is satisfied. 
    \begin{proof}[Proof\textup:\nopunct]
        First of all, it is useful to note that \begin{equation}
            \proposalkernel_\largestepprobability=\largestepprobability\proposalkernel_1+(1-\largestepprobability)\proposalkernel_0.
        \end{equation}
        Now, the transition kernel of the Metropolis-Hastings chain $(\markovchain^\largestepprobability_\discretetimepoint)_{\discretetimepoint\in\discretetimedomain}$ is given by \begin{equation}
            \kernel_\largestepprobability(\point,\measurableset):=\int_\measurableset\proposalkernel_\largestepprobability(\point,\dd{\otherpoint})\acceptancefunction_\largestepprobability(\point,\otherpoint)=\largestepprobability\kernel_1+(1-\largestepprobability)\kernel_0
        \end{equation} for $(\point,\measurableset)\in\measurablespace\times\measurablesystem$, where $\acceptancefunction_\largestepprobability$ is the acceptance function of the Metropolis-Hastings algorithm with proposal kernel $\proposalkernel_\largestepprobability$ and target density $\targetdistribution$ (which effectively does not depend on $\largestepprobability$, whenever the small step kernel $\smallstepkernel$ has a \emph{symmetric} density with respect to the reference measure $\referencemeasure$) and \begin{equation}
            \rejectionprobability_\largestepprobability(\point):=1-\int\proposalkernel_\largestepprobability(\point,\dd{\otherpoint})\acceptancefunction_\largestepprobability(\point,\otherpoint)=\largestepprobability\rejectionprobability_1(\point)+(1-\largestepprobability)\rejectionprobability_0
        \end{equation} for $\point\in\measurablespace$. By definition, the generator of $(\markovchain^\largestepprobability_\discretetimepoint)_{\discretetimepoint\in\discretetimedomain}$ is
        $\localgenerator_\largestepprobability:=\kernel_\largestepprobability-\operatorname{id}_{\measurablesystem_b}$
        % \begin{equation}
        %     \localgenerator_\largestepprobability:=\kernel_\largestepprobability-\operatorname{id}_{\measurablesystem_b}
        % \end{equation}
        and the generator of $(\concatenatedprocess_\timepoint)_{\timepoint\ge0}$ is
        $\concatenatedgenerator=\localgenerator_0+\killingrate\globalgenerator$.
        % \begin{equation}
        %     \concatenatedgenerator=\localgenerator_0+\killingrate\globalgenerator.
        % \end{equation}
        Given that, we obtain \begin{equation}
            \begin{split}
                &\dirichletform(\integrand)-\dirichletform_\largestepprobability(\integrand)=\largestepprobability\dirichletform_0(\integrand)+\expectedlifetime_1\mathcal G(\integrand)-\largestepprobability\dirichletform_1(\integrand)\\&\;\;\;\;\ge \expectedlifetime_1\mathcal G(\integrand)-\largestepprobability\dirichletform_1(\integrand)\\&\;\;\;\;=\expectedlifetime_1\langle\integrand,\integrand-\regenerationdistribution\integrand\rangle_{L^2(\regenerationdistribution)}\\&\;\;\;\;\;\;\;\;\;\;\;\;-\frac\largestepprobability\int\targetdistribution(\dd{\otherpoint})\int\regenerationdistribution(\dd{\otherpoint})\acceptancefunction_\largestepprobability(\point,\otherpoint)\left|\integrand(\point)-\integrand(\otherpoint)\right|^2\\&\;\;\;\;\ge\expectedlifetime_1\langle\integrand,\integrand-\regenerationdistribution\integrand\rangle_{L^2(\regenerationdistribution)}\\&\;\;\;\;\;\;\;\;\;\;\;\;-\frac\largestepprobability{2\targetdensity_\referencemeasure}\int\referencemeasure(\dd{\point})\int\regenerationdistribution(\dd{\otherpoint})\left|\integrand(\point)-\integrand(\otherpoint)\right|^2\\&\;\;\;\;=\left(\expectedlifetime_1-\frac\largestepprobability{2\targetdensity_\referencemeasure}\right)\int\regenerationdistribution(\dd{\point})\int\regenerationdistribution(\dd{\otherpoint})\left|\integrand(\point)-\integrand(\otherpoint)\right|^2\\&\;\;\;\;\;\;\;\;\;\;\;\;+|\regenerationdistribution\integrand|^2-\regenerationdistribution|\integrand|^2
            \end{split}
        \end{equation} for all $\integrand\in\measurablesystem_b$, where \begin{equation}
            \mathcal G(\integrand):=-\langle\integrand,\globalgenerator\integrand\rangle_{L^2(\regenerationdistribution)},
        \end{equation} $\expectedlifetime_1$ is the constant in the definition of the killing rate $\killingrate$, and $\referencemeasure$ and $\targetdensity_\referencemeasure$ are defined as in the main paper. Nothing that $|\regenerationdistribution\integrand|^2-\regenerationdistribution|\integrand|^2$ is the variance of $\integrand$ with respect to the probability measure $\regenerationdistribution$ (hence positive for nontrivial $\integrand$), the claim is immediate from this.
    \end{proof}
\end{theorem}

\onecolumn
\vphantom{\gls{mala}\gls{hmc}\gls{erpt}\gls{rmse}\gls{mrse}\gls{mape}\gls{spp}}
% ----------------------------------------------------------------------------------------------------
% results
% ----------------------------------------------------------------------------------------------------
\section{Additional results and error tables}\label{sec:additional-results}

\begin{figure*}
    \input{figures/kitchen}
    \captionsetup{skip = 0pt}
    \caption{Equal rendering time comparison (60\,s) of Metropolis (left), Metropolis Restore (middle), and \gls{erpt} (right) for the \textsc{Country Kitchen} scene provided by \citep{bitterli2016resources}.}
    \label{fig:kitchen}
\end{figure*}

\input{tables/pool}
\input{tables/veach}
\input{tables/torus}
\input{tables/bathroom}
\input{tables/glass}
\input{tables/kitchen}

% ----------------------------------------------------------------------------------------------------
% bibliography
% ----------------------------------------------------------------------------------------------------
\bibliographystyle{ACM-Reference-Format}
\bibliography{bibliography}

\end{document}
